# Supplementary material for: UAlign: Leveraging Uncertainty Estimations for Factuality Alignment on Large Language Models
Source: arXiv:2412.11803 source file (2025-05-23)
Supplement: Supplementary file 1 [file cases.tex]

\begin{figure*}[!ht]
  \centering
  \includegraphics[width=0.98\textwidth]{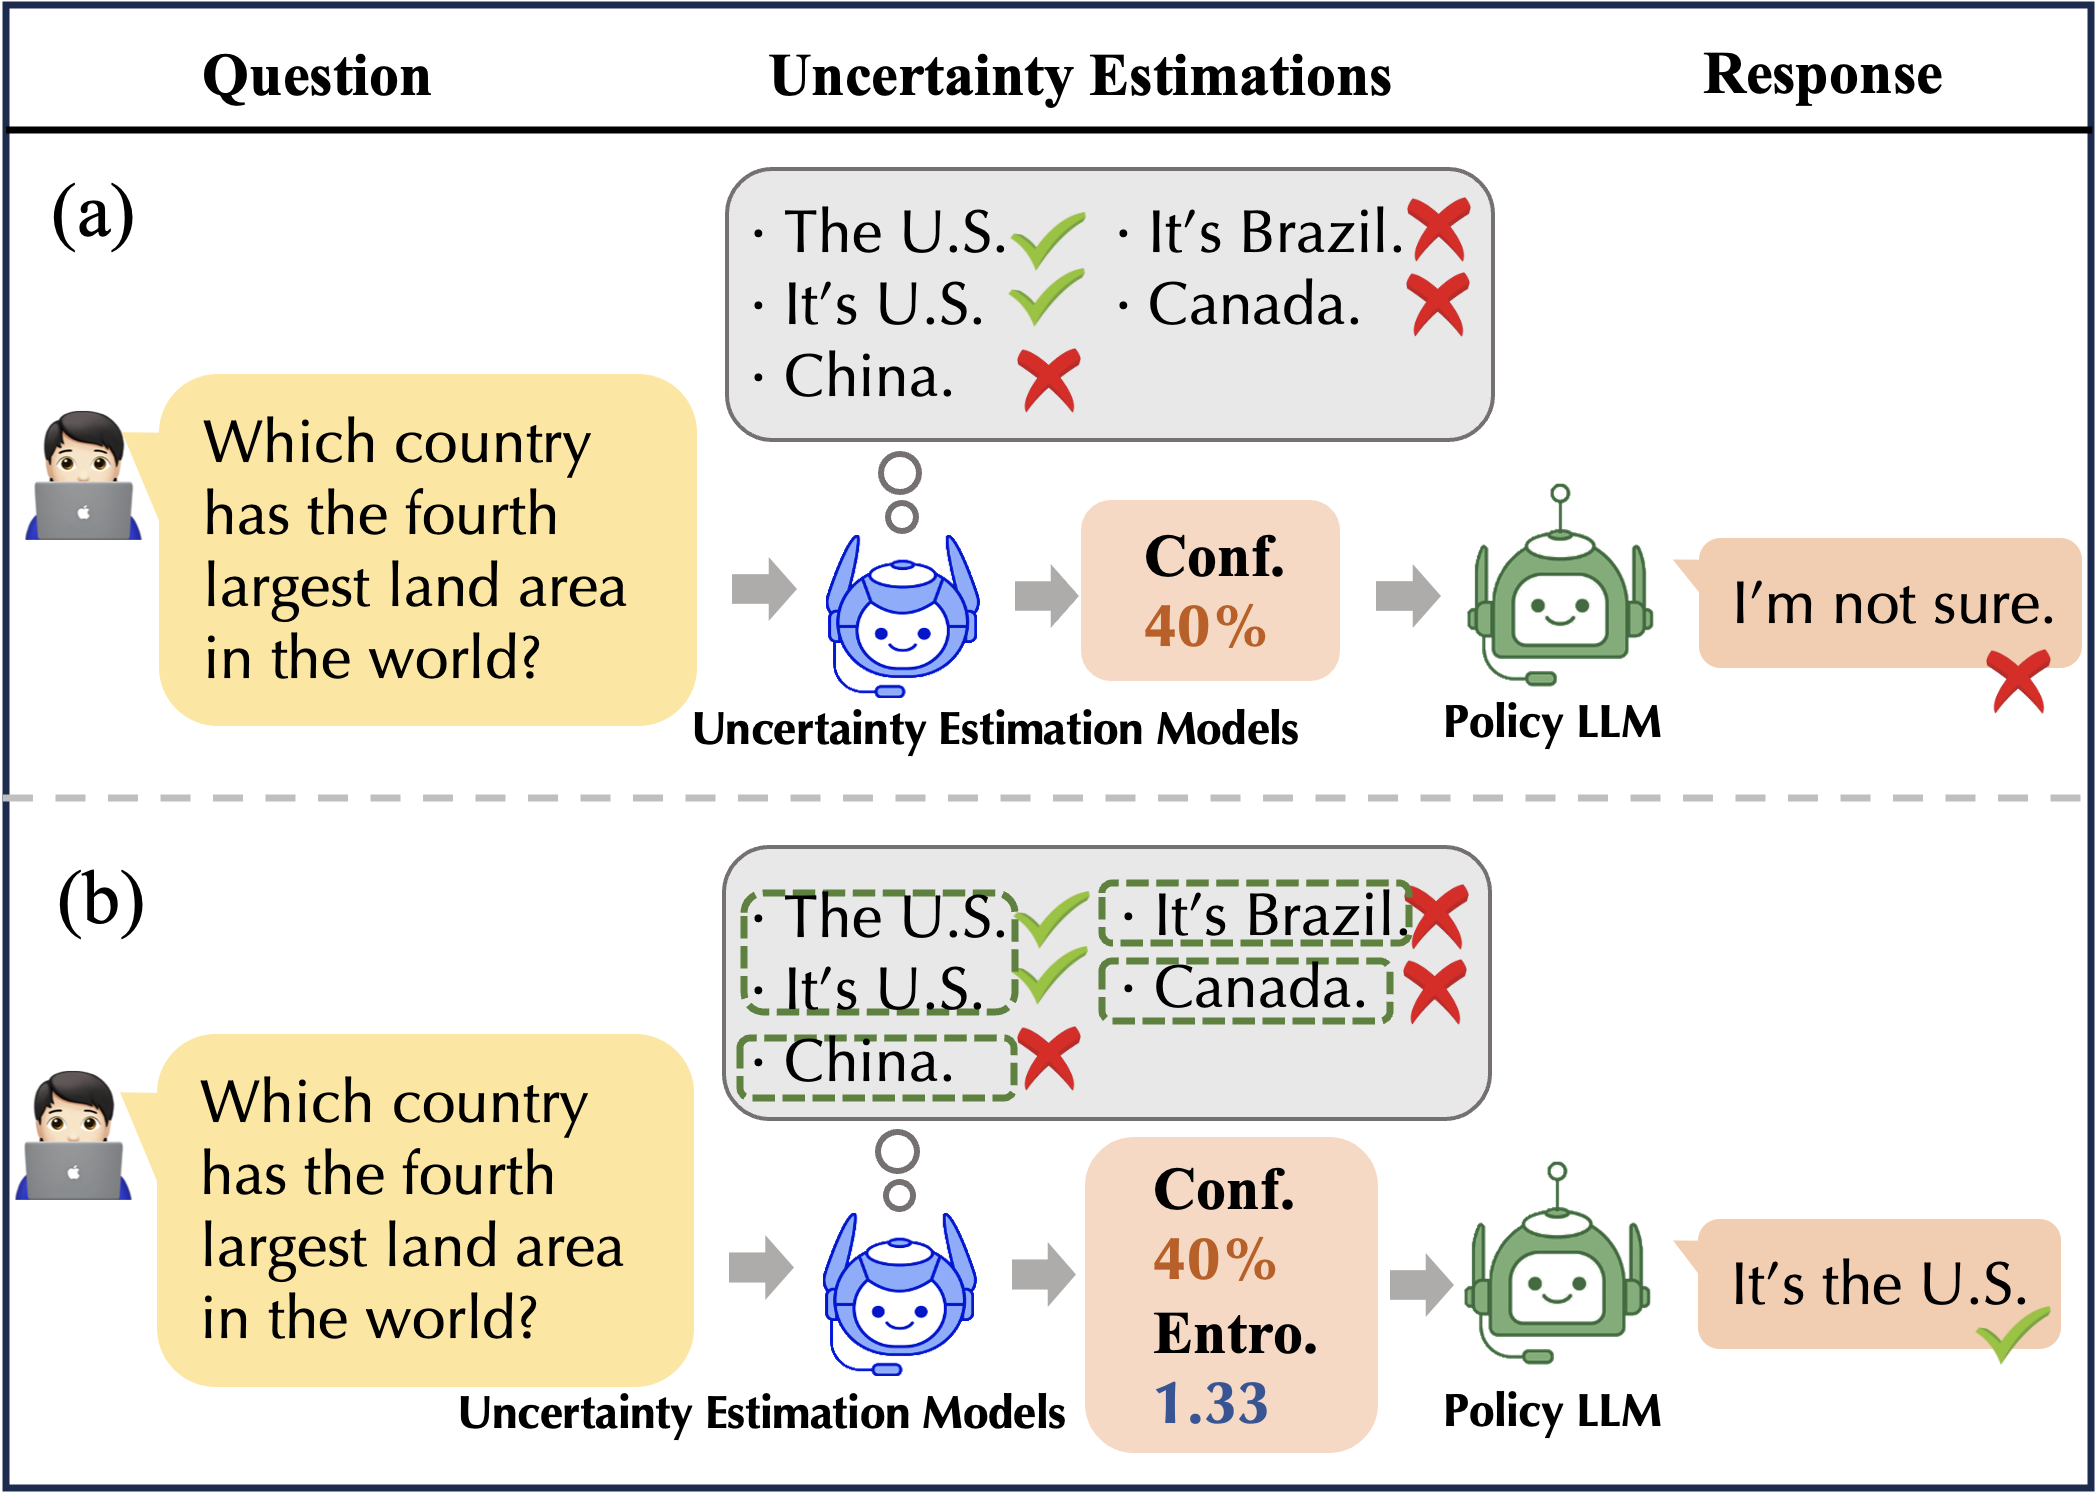}
    \caption{Illustration of effects of different uses of certainty and uncertainty measures under varying knowledge boundaries perceived by LLMs.}
  \label{fig:known}
\end{figure*}
